# Supplementary material for: Risk management with machine-learning-based algorithms
Source: arXiv:1902.05287 source file (2020-08-12)
Supplement: Supplementary file 1 [file appendix.tex]

\appendix
